# Supplementary material for: Particle sizing for flowing colloidal suspensions using flow-differential dynamic microscopy
Source: arXiv:2102.11094 ancillary file (2021-02-22)
Supplement: Supplementary file 1 [file flowDDM_ESI.pdf]

# Supplementary Information: Particle sizing for flowing colloidal suspensions using flow-differential dynamic microscopy

James A. Richards,\* Vincent A. Martinez,\* and Jochen Arlt\*

This supplementary information contains five sections, providing additional information to further support the main text. In §S1 we investigate the impact of the form of the residual velocity distribution, in terms of both the speed distribution and any perpendicular component. In §S2 the depth dependence of flow-DDM for Poiseuille flow is presented; then in §S3, the  $q$  dependence of fits is detailed for both Poiseuille and rheometric flow. Section S4 explicitly explores the extracted velocity distribution as a function of flow speed, before finally in §S5 the behaviour of the far-field correlator is investigated.

## S1 Impact of residual velocity distribution form

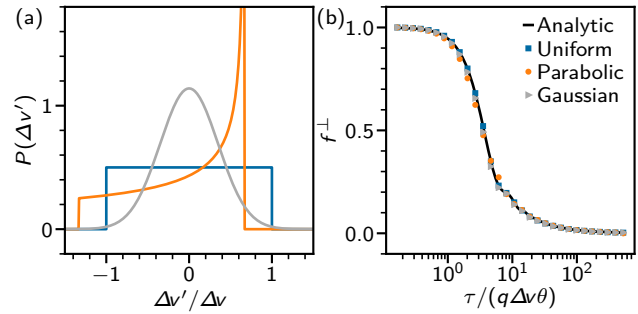

**Fig. S1** Impact of residual velocity distribution form. (a) Residual velocity distributions,  $P(\Delta v')$  for: idealised uniform distribution, blue line; resulting distribution from parabolic flow profile,  $P(\Delta v') = 0.5/\sqrt{2/3 - \Delta v'}$  (orange line); and distribution accounting for contrast variation through optical section using a Gaussian with standard deviation  $0.35\Delta v$ , grey line. (b) Resulting ISF in perpendicular sector,  $f^\perp$ , as a function of reduced delay time,  $\tau/(q\Delta v\theta)$ . Symbols: numerical results, see legend for corresponding  $P(\Delta v')$ . Line: analytic result of Eq. 10 for comparison.

In the main text, analytic results with a uniform velocity distribution,  $P(\Delta v')$ , are presented. This represents an idealisation of experimental conditions, with a simplification of both the flow profile and any intensity variation with depth within the optical section. In Fig. S1 we test the validity of both these assumptions by comparison of the analytic result (Eq. 10) with numerical results using a varying  $P(\Delta v')$ . Significant differences in the form of  $P(\Delta v')$  are seen when considering these complexities. For a uniform section of a parabolic flow profile there is a divergence in the distribution,  $P(\Delta v') = 0.5/\sqrt{2/3 - \Delta v'}$ , Fig. S1(a) (orange line). The divergence originates from the point of the flow profile in which the gradient of the flow velocity is zero. The distribution is also skewed, with a elongated tail towards negative  $\Delta v'$ . We also approximate the variation of image contrast away from the centre of the focal plane with a Gaussian  $P(\Delta v')$ , grey line.

The resultant ISF for the perpendicular sector can be calculated for by numerically integrating Eq. 10 over multiple delay times using the Scipy Python library, Fig. S1 (points). The functional form is almost indistinguishable from the idealised uniform distribution in both the analytic case (line) and numerical solution (blue points). In these results, the width of the Gaussian distribution was adjusted to a standard deviation of  $0.35\Delta v$  to give equivalent decorrelation times. This gives a relation between the full width half maximum and the equivalent  $\Delta v$  extracted from an assumed uniform distribution,  $\text{FWHM} = 0.82\Delta v$ .

Although this complete insensitivity to the exact shape of the velocity distribution might at first sight appear surprising, it is actually a direct consequence of the proposed analysis protocol of flow-DDM. We deliberately choose to examine the dynamics in the direction perpendicular to the flow where it is least sensitive to flow speed (and therefore also the speed distribution along the flow direction). If we were to look parallel to the direction of flow, the dynamics would likely be sensitive to the exact shape of the flow profile, but this is beyond the scope of this study.

So far we have worked on the assumption that the spread in velocities is only along the mean flow direction. Although this is appropriate for simple linear flow geometries, such as the Poiseuille channel flow investigated first, this evidently does not hold in general. Indeed, the rheo-confocal flow investigated in the second part of the manuscript actually has slightly curved flow lines, where the radius of curvature,  $R$ , is set by the distance of the imaged region from the centre of the cone. This leads to a slight variation in the direction of flow throughout the field of view and, therefore, a spread in speed perpendicular to the flow. Here we use a simple

scaling argument to investigate the impact of curvature in such a rotational geometry. A flow with a radius of curvature  $R$  along an image of length  $L_x$  will lead to a residual velocity spread with average magnitude  $v_x L_x / 4R$  in the direction perpendicular to the flow. By comparing decorrelation rates (*i.e.*, timescales), we can approximately determine when diffusion dominates over the flow curvature. This requires  $Dq^2 > qv_x L_x / (4R)$ , or rearranging:  $v_x < 4DqR / L_x$ . For our experimental parameters ( $D = 0.16 \mu\text{m}^2/\text{s}$ ,  $R = 20\text{mm}$ ,  $L_x = 466 \mu\text{m}$  and  $q \approx 2.5 \mu\text{m}^{-1}$ ) this suggests that curvature-induced residual velocities becomes relevant for speeds around  $70 \mu\text{m s}^{-1}$ . This condition is satisfied within the range where we successfully applied flow-DDM (Section 4.2), and therefore it is still (just about) appropriate to treat our rheometric flow data as curvature free. Two aspects of our data support the assertion that this simplified treatment is sufficient: firstly, our finding that the point of failure scales with rate, rather than speed (as would be expected if curvature effects were dominant); and secondly, the absence of strong oscillations in the ISF at and above the maximum shear rate where the diffusivity can be extracted [see Fig. S3(e)] (as would be expected if significant velocities existed in the perpendicular sector, Eq. 6). However, it should be noted that the transverse velocity distribution could easily turn into the dominant decorrelating effect for rheometric flow geometries if conditions are not as carefully chosen, *e.g.* by imaging closer to the cone centre or deeper into the sample.

## S2 Depth dependence in Poiseuille flow

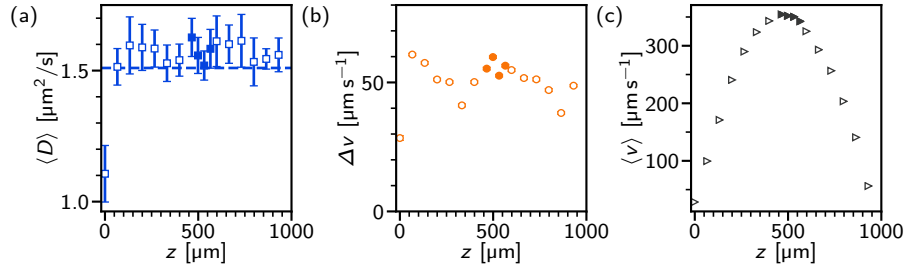

**Fig. S2** Depth dependence in Poiseuille flow for flow-DDM measurement at  $Q = 10 \mu\text{l s}^{-1}$ , corresponding to  $\langle v \rangle \approx 350 \mu\text{m s}^{-1}$  in capillary centre. (a) Extracted diffusion coefficient,  $\langle D \rangle$ , as a function of depth into capillary,  $z$ . Filled symbols, positions used in Fig. 6; open symbols, other positions; and dashed line, rest measurement of  $\langle D \rangle$ . (b) Extracted velocity distribution,  $\Delta v$ . Symbols as in (a). (c) Average drift-velocity,  $\langle v \rangle$ , with changing depth.

At a given flow rate,  $Q = 10 \mu\text{l min}^{-1}$ , flow-DDM measurements can be made across the capillary width ( $z = 0 \mu\text{m}$  to  $1000 \mu\text{m}$ ), Fig. S2(a). The average drift velocity varies across the channel, Fig. S2(c), reaching a maximum of  $\langle v \rangle \approx 350 \mu\text{m s}^{-1}$  in the centre of the capillary;  $z$  positions used in Fig. 6 use filled symbols. This  $\langle v \rangle$  lies within the range for which diffusion can be reliably measured, Fig. 6. Looking across the depth of the capillary at this point, a failure of the technique is seen very near the wall,  $z \approx 0 \mu\text{m}$ , with the drift-corrected ISF in the perpendicular sector no longer diffusive; at such  $z$  an erratic response in  $D(q)$  for standard DDM is also observed. Moving further away from the wall, a consistent  $\langle D \rangle$  is measured across the channel. Similarly, the extracted velocity distribution,  $\Delta v$  [Fig. S2(b)], appears to remain  $\approx 50 \mu\text{m s}^{-1}$ . This suggests that there are multiple contributions to the velocity distribution. For temporal variation in  $Q$  and variation across the width of the channel,  $\Delta v$  would be greatest in the centre of the channel. In contrast, the contribution to  $\Delta v$  from the finite optical section and a velocity gradient in  $z$  is greatest near the walls of the capillary. This suggests that for this combination of imaging and flow geometry that away from the walls there is no preferred depth for minimising  $\Delta v$  due to these multiple contributions. However, for imaging methods with a greater depth of field it would be expected that the centre of the channel would provide the optimal conditions, we therefore focus on the centre of the channel.

## S3 Lengthscale dependence of fitting for flow-DDM

As detailed in Sec. 2, to optimally measure diffusion and size particles it is desirable to access the highest  $q$  (*i.e.* smallest lengthscales) and fit Eqs. 4, 8–12 over the highest  $q$  range possible. This limit may be set by the frame rate,  $Dq_{\text{max}}^2 \approx t_f$ , or (as in this paper) the form factor. We therefore require a  $q$  range where the signal is of a comparable magnitude to the noise, *i.e.*  $A/B > 0.3$ . However,  $A$  and  $B$  are from the fit itself, and are not known *a priori*. Fortunately, in practice these can be estimated from a simple diffusive fit to the perpendicular sector alone (anisotropic-DDM), which allows a determination of the appropriate  $q$  range for flow-DDM.

For full optimisation of the measurements, the  $q$  range would be selected for each movie separately. However, to allow systematic comparison (with, for example, varying flow rate), we fix the  $q$  values used (using half integers) such that  $A/B > 0.3$  for all movies. Example fits from this restricted  $q$  range [ $3.0 \mu\text{m}^{-1}$  to  $3.5 \mu\text{m}^{-1}$  for capillary measurements, grey shading in Fig. S3(c)] are shown at a moderate flow rate [ $Q = 6 \mu\text{l min}^{-1}$  in Fig. S3(a)] and at a high flow rate [ $Q = 60 \mu\text{l min}^{-1}$ , (b)]. At low flow rates the reconstructed ISF is indistinguishable for both sectors ( $\perp/\text{n}\perp$ ) and is diffusive in form. In contrast, at high flow rate the  $\text{n}\perp$  sector decorrelates at a shorter timescale than the  $\perp$  sector and with a steeper slope. In this instance  $f_{\Delta v}$  controls decorrelation for  $\text{n}\perp$  and diffusion for  $\perp$ , demonstrating the sector dependence of the impact of flow that can be used to estimate  $\Delta v$  (and hence whether diffusion is measurable for the  $\perp$ -sector). A fit over a wider  $q$  range ( $1.0 \mu\text{m}^{-1}$  to  $4.0 \mu\text{m}^{-1}$ ) shows that the impact of  $\Delta v$  becomes more important at lower  $q$  [where now  $t_D > t_{\Delta v}/3$  and the fit of  $D(q)$  is erratic and  $> D_0$ ], thus justifying our use of a restricted high  $q$  range.

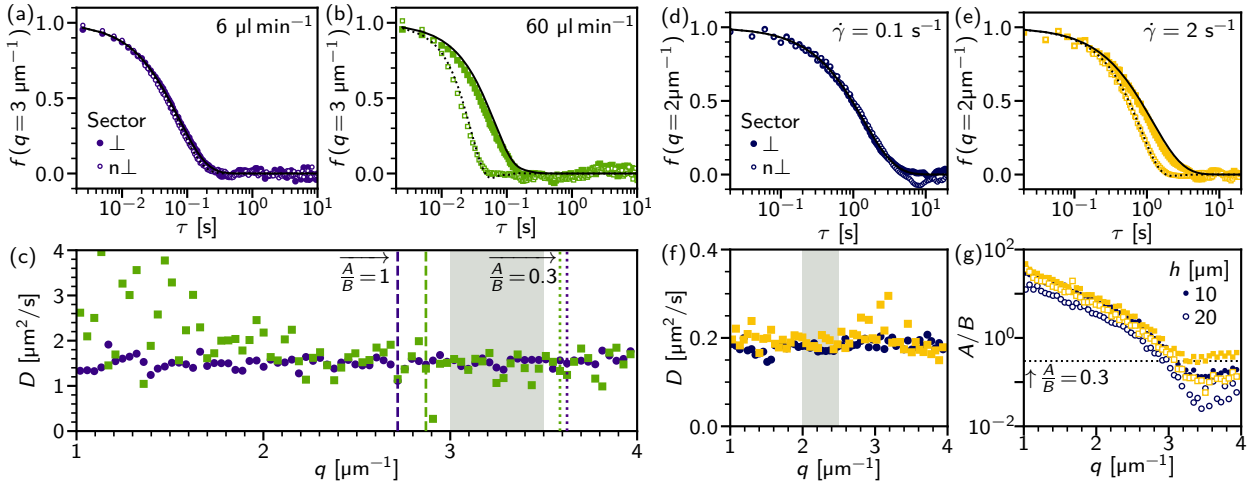

**Fig. S3** DCF fitting and  $q$  dependence. Poiseuille flow: (a) Reconstructed ISF at  $q = 3 \mu\text{m}^{-1}$  with flow rate  $Q = 6 \mu\text{l min}^{-1}$  ( $z = 515 \mu\text{m}$ ). Symbols: filled, perpendicular sector,  $\perp$  ( $\theta = 3^\circ$ ); and, open, adjacent sector,  $n\perp$ . Lines, fit using Eqs. 4, 8–12 over both sectors with  $q = 3.0 \mu\text{m}^{-1}$  to  $3.5 \mu\text{m}^{-1}$  using a single  $\Delta v$  and  $q$ -dependent  $D$ . (b) Reconstructed ISF at high flow rate,  $Q = 60 \mu\text{l min}^{-1}$ , symbols as (a). Lines: solid, fit for perpendicular sector; and, dotted,  $n\perp$  sector. (c)  $q$ -dependent diffusion coefficient,  $D(q)$  over extended fit range  $q = 1.0 \mu\text{m}^{-1}$  to  $4.0 \mu\text{m}^{-1}$ . Symbols: dark (purple) circles,  $Q = 6 \mu\text{l min}^{-1}$ ; and, light (green) squares,  $Q = 60 \mu\text{l min}^{-1}$ . Grey shading,  $q$  range used for  $\langle D \rangle$ . Lines, signal intensity,  $A/B$ , with shade correspondent to  $Q$ : dashed,  $A/B = 1$ ; and, dotted, lower threshold of  $A/B = 0.3$ , all for  $\perp$  sector. Rheometric flow: (d) Reconstructed ISF at  $q = 2 \mu\text{m}^{-1}$  with shear rate  $\dot{\gamma} = 0.1 \text{ s}^{-1}$  ( $h = 10 \mu\text{m}$ ). Symbols and lines as (a),  $\theta = 7.5^\circ$  and  $q = 2.0 \mu\text{m}^{-1}$  to  $2.5 \mu\text{m}^{-1}$ . (e) Reconstructed ISF at high shear rate,  $\dot{\gamma} = 2.0 \text{ s}^{-1}$ . Lines: solid, fit for perpendicular sector; and, dotted,  $n\perp$  sector. (f)  $q$ -dependent diffusion coefficient,  $D(q)$  over extended fit range  $q = 1.0 \mu\text{m}^{-1}$  to  $4.0 \mu\text{m}^{-1}$ . Symbols: dark (blue) circles,  $\dot{\gamma} = 0.1 \text{ s}^{-1}$ ; and, light (yellow) squares,  $\dot{\gamma} = 2.0 \text{ s}^{-1}$ . Grey shading,  $q$  range used for  $\langle D \rangle$ . (g) Signal intensity,  $A/B$  for  $\perp$  sector. Symbols: colours as (d)–(f), filled symbols indicate  $h = 10 \mu\text{m}$  and open symbols  $20 \mu\text{m}$ . Dotted line denotes  $A/B = 0.3$  for  $\perp$  sector.

Similar behaviour is seen with increasing shear rate for rheometric flow, Fig. S3(d) and (e). The  $q$  range was selected using the same process, but note that a lower than desired  $q$  range [ $2.0 \mu\text{m}^{-1}$  to  $2.5 \mu\text{m}^{-1}$ , grey shading in Fig. S3(f)] must be used for images taken at  $h = 10 \mu\text{m}$  to allow an equal comparison with noisier images taken at  $h = 20 \mu\text{m}$  [cf. open and filled symbols in (g)].

## S4 Extracted velocity distribution

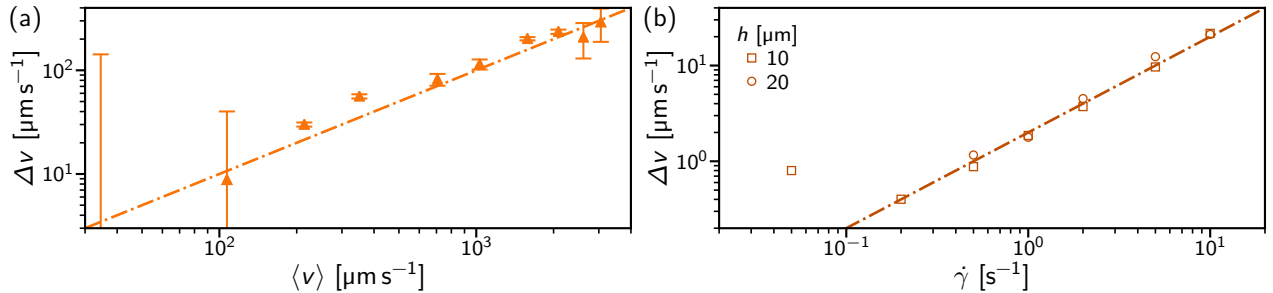

**Fig. S4** Residual velocity distribution with flow speed. (a) Poiseuille flow, extracted velocity distribution width,  $\Delta v$ , as a function of flow speed in the centre of the capillary,  $\langle v \rangle$ . Symbols, average of position, standard deviation given by error bars. (b) Rheo-confocal flow, velocity distribution as a function of applied shear rate,  $\dot{\gamma}$ . Symbols, extracted  $\Delta v$  at different  $h$ , see legend. Line, estimate of linear dependence  $\Delta v = \dot{\gamma} \cdot (2 \mu\text{m})$ .

In the main text we present the decorrelation timescale associated with the velocity distribution extracted from flow-DDM,  $t_{\Delta v}$ , which is of importance in determining the reliability of the diffusivity measurement,  $t_D < t_{\Delta v}/3$ . However, it is also useful to present  $\Delta v$  explicitly as a function of flow speed to make clearer the relation between the velocity distribution and the flow speed or applied shear rate. In Poiseuille flow with averaging over positions in the centre of the capillary, the extracted  $\Delta v$  increases roughly linearly with flow speed, Fig. S4(a) (symbols), although  $\Delta v$  has a high level of error at low flow rates where diffusion dominates. The proportionality (dash-dotted line) gives a velocity distribution  $\Delta v = 0.1 \langle v \rangle$ . For rheometric shear flow, we find that the extracted  $\Delta v$  is proportional to the applied shear rate, Fig. S4(b) (symbols), being independent of the imaging depth,  $h$ . Proportionality,  $\Delta v = 2 \mu\text{m} \cdot \dot{\gamma}$ , implies an optical section of  $1.6 \mu\text{m}$ , using the relation between a uniform  $\Delta v$  and the FWHM, see Sec. S1.

## S5 Far-field dynamic microscopy

In Fig. S5 we show a comparison of the flow-DDM method presented in the main text, (blue) squares, alongside alternate analysis schemes as a function of flow speed. Repeating the flow-DDM analysis but with an increased sector width ( $\theta = 7.5^\circ$ , open triangles)

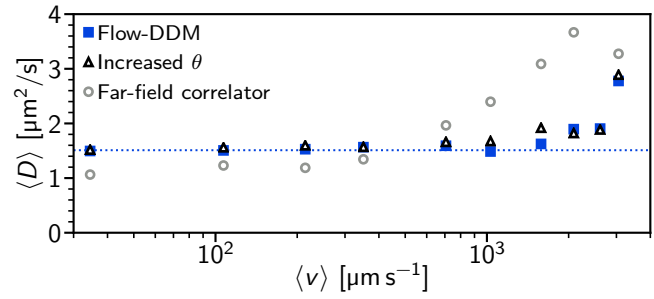

**Fig. S5** Flow rate dependence of alternate diffusivity measurements in Poiseuille flow, averaged diffusion coefficient ( $\langle D \rangle$ ) as a function of flow speed,  $\langle v \rangle$ . Dotted line indicates  $\langle D \rangle = 1.51 \mu\text{m}^2/\text{s}$  measured at rest, Fig. 4(a). Symbols: filled (blue) squares, flow-DDM with sector width  $\theta = 3^\circ$  and  $q$  range  $3.0 \mu\text{m}^{-1}$  to  $3.5 \mu\text{m}^{-1}$ , as in Fig. 6(a); open (black) triangles, flow-DDM with increased sector width,  $\theta = 7.5^\circ$ ; and, open (grey) circles, far-field dynamic microscopy with  $\theta = 3^\circ$  and  $q = 2.0 \mu\text{m}^{-1}$  to  $2.5 \mu\text{m}^{-1}$ .

shows the influence of flow at lower speeds. This arises from the larger residual velocity components included in the broader sector, with a clear increase in the measured  $\langle D \rangle$  at  $\langle v \rangle = 1000 \mu\text{m s}^{-1}$ .

An alternate digital Fourier microscopy method for samples being deformed has been suggested by Aime and Cipelletti<sup>1</sup>. This “far-field” dynamic microscopy (FFDM) uses a higher-order correlator that in ideal conditions measures the square of the magnitude of the ISF,  $|f|^2$ . Being dependent only on the magnitude of the ISF (in place of the real part alone, as with DDM), such a correlator is independent of the phase and thus any global translation of the sample. Applying FFDM should conceptually be equal to the drift correction applied in Sec. 2. However, we find in quiescent samples that FFDM is inconsistent with DDM, with a lower diffusivity measured for both imaging methods, Fig. S6(a) and (b). In flowing samples, the diffusivity measured from a perpendicular sector ( $\theta = 3^\circ$ ) at the highest accessible  $q$  range ( $2.0 \mu\text{m}^{-1}$  to  $2.5 \mu\text{m}^{-1}$ ) increases at lower flow rates than flow-DDM (Fig. S5), instead the increase is comparable to that in anisotropic-DDM, Fig. 6. Together, these indicate that for the microscopy methods used (and also likely movies taken of industrially relevant samples) FFDM is impacted by cross-terms in the higher-order correlator. When considering such cross terms between signal and noise the correlator is no longer invariant to a global translation, with a mix of  $|f|^2$  and  $f$  terms that is not amenable to a simple interpretation. This link between signal and noise is seen in  $A(q)$  and  $B(q)$ , Fig. S6(c) and (d), cf. light (grey) and dark (blue) symbols.

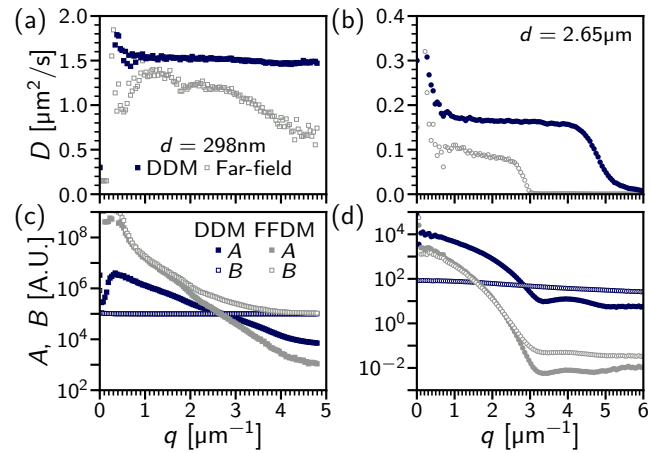

**Fig. S6** Comparison of Fourier Digital Microscopy methods for diffusion measurements of quiescent samples. (a) Phase-contrast microscopy of a dilute suspension of 300 nm polystyrene particles as a function of wavevector,  $q$ . Symbols: filled dark (blue) squares, DDM; light (grey) open squares, “far-field” correlator (FFDM). (b) Confocal microscopy of a dilute colloidal suspension, PMMA in density-matched CsCl solution (with Hanning window applied). Symbols,  $D(q)$  for: filled (blue) circles, DDM; open (grey) circles, FFDM. (c) Signal [filled,  $A(q)$ ] and noise [open,  $B(q)$ ] for  $D$  measurements in (a), symbols and colours as in (a). (d)  $A(q)$  and  $B(q)$  for measurements in (b), with colouring as in (c).

## Notes and references

- 1 S. Aime and L. Cipelletti, *Soft Matter*, 2019, **15**, 213–226.
